# Supplementary material for: Auto-Regressive Models Need Structural Registers: Semantic Foresight Improves Coherent Driving Video Continuation
Source: arXiv:2412.03758 source file (2026-10-06)
Supplement: Supplementary file 1 [file X_suppl.tex]

\clearpage
\setcounter{page}{1}
\maketitlesupplementary

\begin{figure*}
    \centering
    \includegraphics[width=1.0\linewidth]{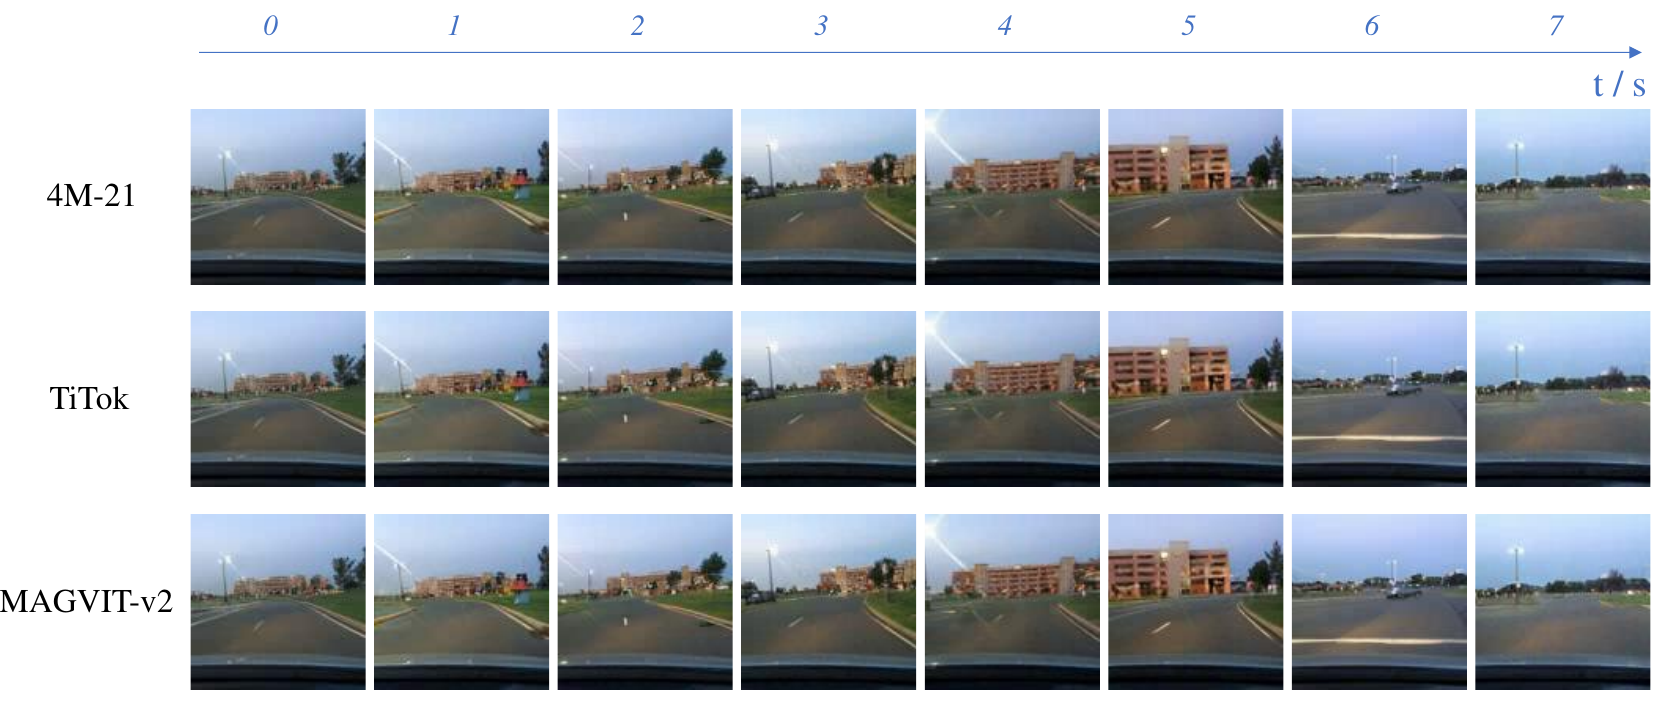}
    \caption{Reconstruction of different tokenizers.}
    \label{fig:rec}
\end{figure*}

% 对于生成模型来说，一个合适的tokenizer需要考虑很多因素，包括码率、重建质量、码表大小等等，在这里我们讨论最先进的几种image tokenizer。不同的tokenizer有不同的设计理念，4m-21希望通过多模态数据对齐使tokenizer携带更多的高级语义信息，titok希望尽可能压缩tokenizer的码率，Magvit-v2希望以非常大的词表实现尽可能高的重建质量。这些tokenizer做视频重建任务的效果见图。

For generative models, a suitable visual tokenizer needs to consider many factors, including coding rate, reconstruction quality, codebook size, etc. Here we discuss several state-of-the-art image tokenizers. Different tokenizers have different design philosophies, 4M-21~\cite{bachmann20244m} wants to make the tokenizer carry more high-level information through multimodal data alignment, TiTok~\cite{yu2024image} wants to compress the tokenizer's bit rate as much as possible, and MAGVIT-v2~\cite{yu2023language} wants to achieve the highest possible reconstruction quality with a very large word list. The results of these tokenizers tackling the video reconstruction task are shown in \cref{fig:rec}.
